# Supplementary material for: MobileDev-Bench: A Benchmark for Issue Resolution in Mobile Application Development
Source: arXiv:2603.24946 source file (2026-05-08)
Supplement: Supplementary file 1 [file appendix_evaluations.tex]

\section{Evaluation}
\label{sec:appendix_evaluation}

In this section, we evaluate MobileDev-Bench by measuring how well state-of-the-art language models can automatically repair real-world mobile development issues. Our evaluation addresses two research questions: (1) Can frontier models localize and repair bugs across diverse mobile frameworks (Android, Flutter, React Native)? (2) How does model performance vary across programming languages and repository characteristics? We assess four recent frontier models using established code repair metrics, providing the first systematic comparison of automated program repair capabilities on mobile-specific codebases. \todo{continue from here}

\subsection{Experimental Setup}

\subsubsection{Evaluation Framework}

We evaluate MobileDev-Bench using the localization and repair phases from Agentless~\citep{xia2024agentless}, a state-of-the-art autonomous code repair framework. Agentless decomposes the repair task into: (1) fault localization, where the model identifies potentially buggy files and functions using the issue description and repository context, and (2) patch generation, where the model produces a unified diff targeting the localized elements. We validate generated patches using our own test harness, which applies each patch to the base commit and executes the repository's test suite to determine whether the repair resolves the issue. This approach mirrors the workflow of Multi-SWE-bench evaluation and enables direct comparison with existing benchmarks while avoiding the compounding errors of full agentic systems.

In our adaptation, similar to MagentLess,\footnote{\url{https://github.com/multi-swe-bench/MagentLess}} we incorporate tree-sitter\footnote{\url{https://pypi.org/project/tree-sitter-language-pack/}} for parsing and extracting code structures across Java, Kotlin, TypeScript, and Dart, replacing the AST-based approach used for Python in the original Agentless implementation. This enables robust syntactic analysis across the diverse mobile development languages in our benchmark.

\subsubsection{Model Selection}

We evaluate four frontier language models representing diverse architectural approaches and training regimes: Claude Sonnet 4.5~\citep{anthropic2025claude}, GPT-5.2~\citep{openai2025gpt52}, Gemini 2.5 Flash~\citep{comanici2025gemini25pushingfrontier}, and Qwen-3-Coder~\citep{qwen2025qwen3coder}. Claude Sonnet 4.5 and GPT-5.2 are proprietary models with large context windows and strong code generation capabilities. Gemini 2.5 Flash prioritizes low-latency inference with native multimodal support. Qwen-3-Coder is an open-weight model fine-tuned specifically for code completion and repair tasks.
%, providing a non-proprietary baseline for reproducibility. 
To ensure fair comparison and deterministic patch generation, we disable extended reasoning modes where available (setting \texttt{reasoning\_effort=low} for GPT-5.2 and omitting thinking budgets for Claude Sonnet 4.5), following the original Agentless~\citep{xia2024agentless} evaluation protocol design.
% before such features existed.

% \subsubsection{Evaluation Metrics}

% Following prior work~\citep{xia2024agentless}, we report two complementary metrics that separately assess repair capability and localization accuracy:

% % repair skill (resolution rate) vs. localization skill (localization rate)

% \textbf{\% Resolved.} The percentage of instances where the model-generated patch passes all tests when applied to the base commit, achieving the same test outcomes as the ground truth developer patch. This metric captures end-to-end repair capability.

% \textbf{Recall.} The fraction of ground truth patch locations that appear in the model-generated patch:
% \[
% \text{Recall} = \frac{|\text{Ground Truth Locations} \cap \text{Predicted Locations}|}{|\text{Ground Truth Locations}|}
% \]
% This metric isolates fault localization performance independent of patch correctness.

% These metrics distinguish between localization skill (can the model identify where to edit?) and repair skill (can the model generate a correct fix?). High Recall with low \% Resolved indicates strong localization but weak code generation. Conversely, low Recall bounds the maximum achievable \% Resolved, as a model cannot repair code it fails to locate.

\subsubsection{Metrics}

Following prior work~\citep{xia2024agentless, 2025swepolybench}, we report two complementary metrics that separately assess repair capability and localization accuracy.

\textbf{Resolution Rate.} Let $T$ denote the total number of tasks. For each task $t$, we define $\mathbf{1}(\mathrm{Pass}_t)$ as an indicator function that equals 1 if the model-generated patch passes all tests when applied to the base commit, and 0 otherwise. We compute Resolution Rate as:
\[
\mathrm{Resolution\ Rate} =
\frac{1}{T} \sum_{t=1}^{T} \mathbf{1}(\mathrm{Pass}_t)
\]
This metric measures end-to-end repair capability at the task level.

\vspace{5pt}

\textbf{Retrieval scores.} For each task $t$, let $F^{GT}_t$ denote the set of ground truth modified files and let $F^{Pred}_t$ denote the set of files modified by the model-generated patch. We compute file-level retrieval metrics per task as:
\begin{align*}
\mathrm{Recall}_t &= \frac{|F^{GT}_t \cap F^{Pred}_t|}{|F^{GT}_t|} \\
\mathrm{Precision}_t &= \frac{|F^{GT}_t \cap F^{Pred}_t|}{|F^{Pred}_t|} \\
\mathrm{F1}_t &= \frac{2 \cdot \mathrm{Precision}_t \cdot \mathrm{Recall}_t}{\mathrm{Precision}_t + \mathrm{Recall}_t}
\end{align*}
We then report macro-averaged metrics across all $T$ tasks:
\begin{align*}
\mathrm{Recall} &= \frac{1}{T} \sum_{t=1}^{T} \mathrm{Recall}_t \\
\mathrm{Precision} &= \frac{1}{T} \sum_{t=1}^{T} \mathrm{Precision}_t \\
\mathrm{F1} &= \frac{1}{T} \sum_{t=1}^{T} \mathrm{F1}_t
\end{align*}
These metrics measure fault localization performance independently of patch correctness. Recall captures the fraction of ground truth files correctly identified, while Precision measures the fraction of predicted files that are actually relevant. F1 provides a harmonic mean balancing both aspects. Together with Resolution Rate, these metrics distinguish localization capability from repair capability. High recall with low Resolution Rate suggests that the model identifies the correct files but fails to generate correct fixes. Conversely, low recall limits achievable Resolution Rate, since a model cannot repair files it does not localize. High precision indicates the model avoids over-editing irrelevant files.

% mobile development doesn't map cleanly onto the granularity levels inherited from Python-centric benchmarks, and that's part of what makes MobileDev-Bench a distinct contribution.

% granularity levels:

% module-level: 
% - exclude single-module repos from this metric, or note it as "N/A" for those instances
% file-level:
% function-level: 
% - Flutter code is declarative UI building inside build() methods, exclude Flutter instances from function-level reporting or treat widget classes as the equivalent unit.
% - For patches touching non-code files, function-level granularity is simply undefined.
% line-level:

% NOTE: we compute function and line level metrics over code-only patches (Kotlin/Java/Dart files), and report file-level for everything

\subsection{Results}

We evaluate four frontier models on MobileDev-Bench's task instances, measuring both fault localization capability (file-level retrieval metrics) and end-to-end repair performance (resolution rate). Table~\ref{tab:resolution-rate} shows the resolution rates, and Table~\ref{tab:retrieval-metrics} presents the retrieval metrics.

\input{table_resolution_rate}

\subsubsection{Resolution Rate Overview}

Table~\ref{tab:resolution-rate} shows resolution rates for both settings on 415 verified tasks.
Rate is computed as resolved / evaluated, where evaluated excludes instances with no submitted prediction (Agentless) or an empty patch (Oracle).
Under the Agentless setting, rates are low and tightly clustered, ranging from 3.90\% (GPT-5.2, 16/410) to 4.28\% (Qwen3 Coder, 17/397).
Under the Oracle setting---where ground-truth files are provided directly---rates diverge more widely, from 1.94\% (Gemini 2.5 Flash, 8/412) to 6.07\% (Claude Sonnet 4.5, 25/412).
The consistent gap between Oracle and Agentless rates confirms that fault localization is a primary bottleneck; even with ground-truth files provided, patch generation on multi-file mobile tasks remains difficult.

The 32 unique Agentless resolved instances (some resolved by multiple models) exhibit distinct patterns when analyzed by artifact type diversity, file count, and programming language (Table~\ref{tab:resolution-rate-breakdown}).

\input{table_resolution_rate_detailed}

\subsubsection{Artifact Type Diversity and Resolution Success}

Single-artifact tasks show substantially higher resolution rates than multi-artifact tasks. While only 57.8\% of benchmark tasks modify a single artifact type (Source, Resource, i18n, Build, or Manifest), 84.4\% of resolved Agentless instances are single-artifact changes. This represents a 1.46x overrepresentation, indicating models are significantly more successful when changes remain within a single artifact category.

Conversely, multi-artifact tasks requiring coordinated changes across different artifact types account for 42.2\% of the benchmark but only 15.6\% of resolutions (0.37x ratio). This gap highlights a fundamental limitation in current models' ability to coordinate changes across heterogeneous file types. For instance, tasks requiring simultaneous updates to source code, build configuration, and resource files present coordination challenges that models struggle to address. The difficulty stems from understanding dependencies between artifact types. A change to a Gradle build file enabling a new feature flag must be paired with corresponding source code modifications and potentially resource file updates. Models frequently identify changes in one artifact type but fail to propagate necessary modifications to related artifacts.

\subsubsection{File Count as a Resolution Predictor}

File count strongly predicts resolution likelihood, though the relationship is non-monotonic. Single-file tasks comprise 17.1\% of the benchmark but 65.6\% of Agentless resolutions, a 3.84x overrepresentation. This dramatic skew demonstrates that models excel at isolated, single-location fixes where fault localization reduces to identifying one file and patch generation requires modifying only that file.

Tasks requiring 2--3 files show near-proportional representation (15.6\% of resolutions vs. 21.4\% of benchmark, 0.73x ratio), suggesting models handle small multi-file changes reasonably well when the files are closely related. However, mid-range complexity tasks with 4--5 files and 6--10 files are severely underrepresented (6.3\% and 0.0\% of resolutions vs. 12.5\% and 16.9\% of benchmark, 0.50x and 0.00x ratios respectively). These tasks represent a difficulty cliff where models must track multiple interconnected changes but lack the regularity patterns that aid in very large refactorings.

Interestingly, tasks requiring 11+ files account for 12.5\% of Agentless resolutions despite representing 32.1\% of the benchmark (0.39x ratio). While still underrepresented, this is a smaller gap than the mid-range file counts. Analysis of resolved instances with 11+ files reveals this modest recovery is primarily repository-specific rather than pattern-driven. The majority come from \texttt{element-hq/element-x-android}, suggesting certain codebases may have architectural characteristics that facilitate large-scale automated changes. These instances represent genuine multi-module refactorings with consistent structure and comprehensive test coverage, rather than simple mechanical changes like i18n file updates.

Resolution rates exhibit a non-monotonic relationship with file count. Very simple tasks (1 file) achieve the highest success (12-15\%), while mid-complexity tasks (4-10 files) prove most challenging with near-zero resolution rates (0-2\%). Tasks requiring 11+ files show modest recovery (0.0-4.2\%), though this appears driven by repository-specific factors (particularly element-x-android) rather than general properties of large-scale changes.

\subsubsection{Language-Independent Difficulty Patterns}

\input{table_retrieval_metrics}

Language distribution among resolved instances shows variation across the four languages represented in MobileDev-Bench. Kotlin tasks, comprising 78.6\% of the benchmark, account for 71.9\% of Agentless resolutions (0.91x ratio), indicating near-proportional resolution success. Dart tasks show notable overrepresentation at 28.1\% of resolutions versus 15.2\% of the benchmark (1.85x ratio), while TypeScript tasks are substantially underrepresented at 0.0\% of resolutions versus 4.1\% of the benchmark (0.00x ratio). Strikingly, Java tasks (2.2\% of benchmark, representing only AntennaPod repository) achieved zero resolutions across all models (0.00x ratio).

The mixed language results warrant careful interpretation. Kotlin's near-proportional success and Java's complete failure, despite both being Android languages, suggests factors beyond mere language syntax. AntennaPod, the sole Java repository in MobileDev-Bench, may represent an older codebase with different architectural patterns compared to the modern Kotlin-based Android projects. Dart's overperformance (1.85x) indicates Flutter tasks may be somewhat more amenable to automated repair, possibly due to framework conventions or task characteristics in the talawa and zulip-flutter repositories. TypeScript's underperformance (0.00x) may reflect the complexity of React Native's JavaScript-native bridge architecture.

Despite these variations, the overall pattern suggests task complexity remains the dominant factor. The core challenges, fault localization across multiple files and coordination of heterogeneous artifacts, manifest across all four languages. Whether working with Kotlin/Java Android projects, Dart Flutter applications, or TypeScript React Native apps, models face fundamental difficulties identifying all necessary modification sites and generating coherent multi-file patches. This finding suggests that improvements to model architectures for program repair should prioritize general capabilities for multi-file reasoning and cross-artifact coordination, while also investigating language-specific patterns that may explain the observed differences.

\subsubsection{Fault Localization Performance}

File-level recall varies from 13.5\% to 18.3\% across models, with Claude Sonnet 4.5 achieving the highest score. However, models show much higher precision (42--58\%), indicating they are conservative in their file modifications. When they edit a file, it is usually relevant, but they miss many ground truth files. The resulting F1 scores (17.3--23.0\%) balance these complementary aspects. These metrics reveal that fault localization, not patch generation, is the primary bottleneck for automated mobile app repair. Models struggle to identify which files need modification, even when they can generate syntactically valid code changes.

We observe three distinct recall patterns across the benchmark:

\textbf{Perfect localization (Recall = 1.0)} occurs in 5--8\% of tasks, almost exclusively on single-file changes. These tasks typically involve isolated bug fixes within a single module where all models correctly identify the sole file requiring modification.

\textbf{Zero localization (Recall = 0.0)} affects 46--59\% of tasks, where models modify entirely incorrect files. For example, when the ground truth patch modifies internationalization resource files, 
% (\texttt{lang/*.json}),
models frequently predict changes to source code files instead. This pattern suggests models over-focus on source code and miss non-code artifacts. Notably, 162 tasks (29\%) exhibit zero recall across all four models, indicating consistently challenging instances.

\textbf{Partial localization (0 < Recall < 1)} represents 36--47\% of tasks. Models identify some but not all relevant files. For instance, in tasks requiring 9 ground truth files, models typically find only 2 files (22\% recall). This pattern is common in multi-module changes where models correctly localize the primary bug location but miss cascading modifications in related modules, services, or UI layers.

\subsubsection{Multi-File Changes Drive Localization Difficulty}

Mobile development tasks frequently require coordinated changes across multiple files. On average, ground truth patches in MobileDev-Bench modify 13.5 files per task (median: 5 files), dramatically higher than Python-centric benchmarks like SWE-bench (1.3 files per task). Only 17.1\% of tasks (71/415) involve single-file changes, while 82.9\% require modifications across multiple files.

This multi-file nature directly impacts localization performance. Table~\ref{tab:retrieval-metrics} shows how all three metrics degrade as the number of ground truth files increases. Single-file tasks achieve 35--55\% recall across models, but multi-file tasks drop to 7--9\% recall for 6--10 file tasks, a gap of 26--48 percentage points. The best-performing model (Claude Sonnet 4.5) achieves 54.9\% recall on single-file tasks but only 3.0\% recall on tasks requiring 11+ file modifications. Interestingly, precision increases with file count (from 34--53\% on single-file tasks to 48--68\% on 6--10 file tasks), suggesting models become more conservative when facing complex multi-file changes.

This performance gap highlights a fundamental architectural difference between mobile and server-side development. Mobile apps organize functionality across modules (Gradle/build system), services (business logic), view models (state management), UI widgets (presentation), and resource files (layouts, strings, configurations). A single user-facing bug often requires coordinated changes across these layers. For instance, adding a new API field may necessitate updates to the API client, domain model, view model, UI component, and test fixtures. Current models fail to trace these cross-cutting dependencies, achieving near-zero recall on such tasks.

\subsubsection{Implications for Resolution Rate}

The low recall scores impose an upper bound on achievable resolution rates. Since models cannot repair files they fail to localize, even perfect patch generation for correctly identified files would yield at most 13--18\% resolution rate (matching the recall ceiling). In practice, resolution rates must be lower, as models must both (1) localize all relevant files \textit{and} (2) generate correct fixes for those files.

This finding inverts the traditional assumption in automated program repair that patch generation is the primary challenge. For mobile development tasks in MobileDev-Bench, localization is the dominant failure mode.
